# Supplementary material for: The Future of Open Human Feedback
Source: arXiv:2408.16961 source file (2024-09-04)
Supplement: Supplementary file 1 [file appendix.tex]

\newpage
\appendix
\section{On feedback data card}\label{ap:card}
Contributors will be asked to provide the following information in the data card (similar to other data cards and datasheets \citep{shimorina2021human,pushkarna2022data}):
Dataset overview: Title, description, source, license, and any relevant publications or blog posts. Motivation and composition: The reasons behind creating the dataset, what it contains (data types, features, etc.), and how it is structured. Collection process: Detailed description of how the data was collected, including tools, techniques, and ethical considerations (e.g., Institutional Review Board [IRB] approval if applicable). Preprocessing and cleaning: Any steps taken to clean, normalize, or transform the data before making it available. Intended use and potential applications: The original purpose of the data collection, as well as any potential research questions or use cases it could address. Uses and limitations: Description of how the data is intended to be used, as well as any known biases or limitations that users should be aware of.
Maintenance: Information about how the dataset will be updated or maintained over time. Provenance and licensing information: Clear documentation of the data's origin, including any relevant licenses or usage restrictions.

The data card itself, along with any associated documentation (e.g., research papers, technical documentation), will be governed by the Creative Commons Attribution (CC BY) license. This open license allows others to freely share, adapt, and build upon the documentation, as long as they give appropriate credit to the original contributor (possibly in the proper hashed way chosen see \S\ref{sec:privacy}).
